# Supplementary material for: Gaze-Guided 3D Hand Motion Prediction for Detecting Intent in Egocentric Grasping Tasks
Source: arXiv:2504.01024 source file (2025-03-27)
Supplement: Supplementary file 1 [file 07_appendix.tex]

\section*{APPENDIX}

\begin{figure*}[htpb]

\begin{subfigure}{0.32\textwidth}
  \includegraphics[width=\linewidth]{figures/pred_map/bottleB22.pdf}
\end{subfigure}\hfill
\begin{subfigure}{0.32\textwidth}
  \includegraphics[width=\linewidth]{figures/pred_map/bottleD04.pdf}
\end{subfigure}\hfill
\begin{subfigure}{0.32\textwidth}
  \includegraphics[width=\linewidth]{figures/pred_map/bottleP03.pdf}
\end{subfigure}
\caption{Bottle}
\medskip

\begin{subfigure}{0.32\textwidth}
  \includegraphics[width=\linewidth]{figures/pred_map/earphoneD19.pdf}
\end{subfigure}\hfill
\begin{subfigure}{0.32\textwidth}
  \includegraphics[width=\linewidth]{figures/pred_map/earphoneD20.pdf}
\end{subfigure}\hfill
\begin{subfigure}{0.32\textwidth}
  \includegraphics[width=\linewidth]{figures/pred_map/earphoneD21.pdf}
\end{subfigure}
\caption{Earphone}
\medskip

\begin{subfigure}{0.32\textwidth}
  \includegraphics[width=\linewidth]{figures/pred_map/paperG07.pdf}
\end{subfigure}\hfill
\begin{subfigure}{0.32\textwidth}
  \includegraphics[width=\linewidth]{figures/pred_map/paperL07.pdf}
\end{subfigure}\hfill
\begin{subfigure}{0.32\textwidth}
  \includegraphics[width=\linewidth]{figures/pred_map/paperO22.pdf}
\end{subfigure}
\caption{Paper}
\medskip

\begin{subfigure}{0.32\textwidth}
  \includegraphics[width=\linewidth]{figures/pred_map/penB14.pdf}
\end{subfigure}\hfill
\begin{subfigure}{0.32\textwidth}
  \includegraphics[width=\linewidth]{figures/pred_map/penG29.pdf}
\end{subfigure}\hfill
\begin{subfigure}{0.32\textwidth}
  \includegraphics[width=\linewidth]{figures/pred_map/penH30.pdf}
\end{subfigure}
\caption{Pen}
\medskip

\begin{subfigure}{0.32\textwidth}
  \includegraphics[width=\linewidth]{figures/pred_map/phoneB18.pdf}
\end{subfigure}\hfill
\begin{subfigure}{0.32\textwidth}
  \includegraphics[width=\linewidth]{figures/pred_map/phoneD15.pdf}
\end{subfigure}\hfill
\begin{subfigure}{0.32\textwidth}
  \includegraphics[width=\linewidth]{figures/pred_map/phoneD16.pdf}
\end{subfigure}
\caption{Phone}
\medskip

\end{figure*}
visualization of predicted hand pose

left and right hand result (if add this in appendix, also discuss this result in discussion part)

Additionally, we calculate the key-pose angle error to assess the trajectory alignment relative to the intended target. This error measures the angle between vectors extending from the starting point to the ground truth and to the prediction, respectively. As illustrated in Fig. \ref{res_angle}, the trends in angle error for models with and without gaze are consistent with those observed in distance error. Generally, the model incorporating gaze demonstrates lower-angle errors across all three groups, with a few exceptions. This finding suggests that integrating eye gaze into the model improves path efficiency.

% angle error
\begin{figure*}[htbp]
\centering
\includegraphics[width=0.95\textwidth]{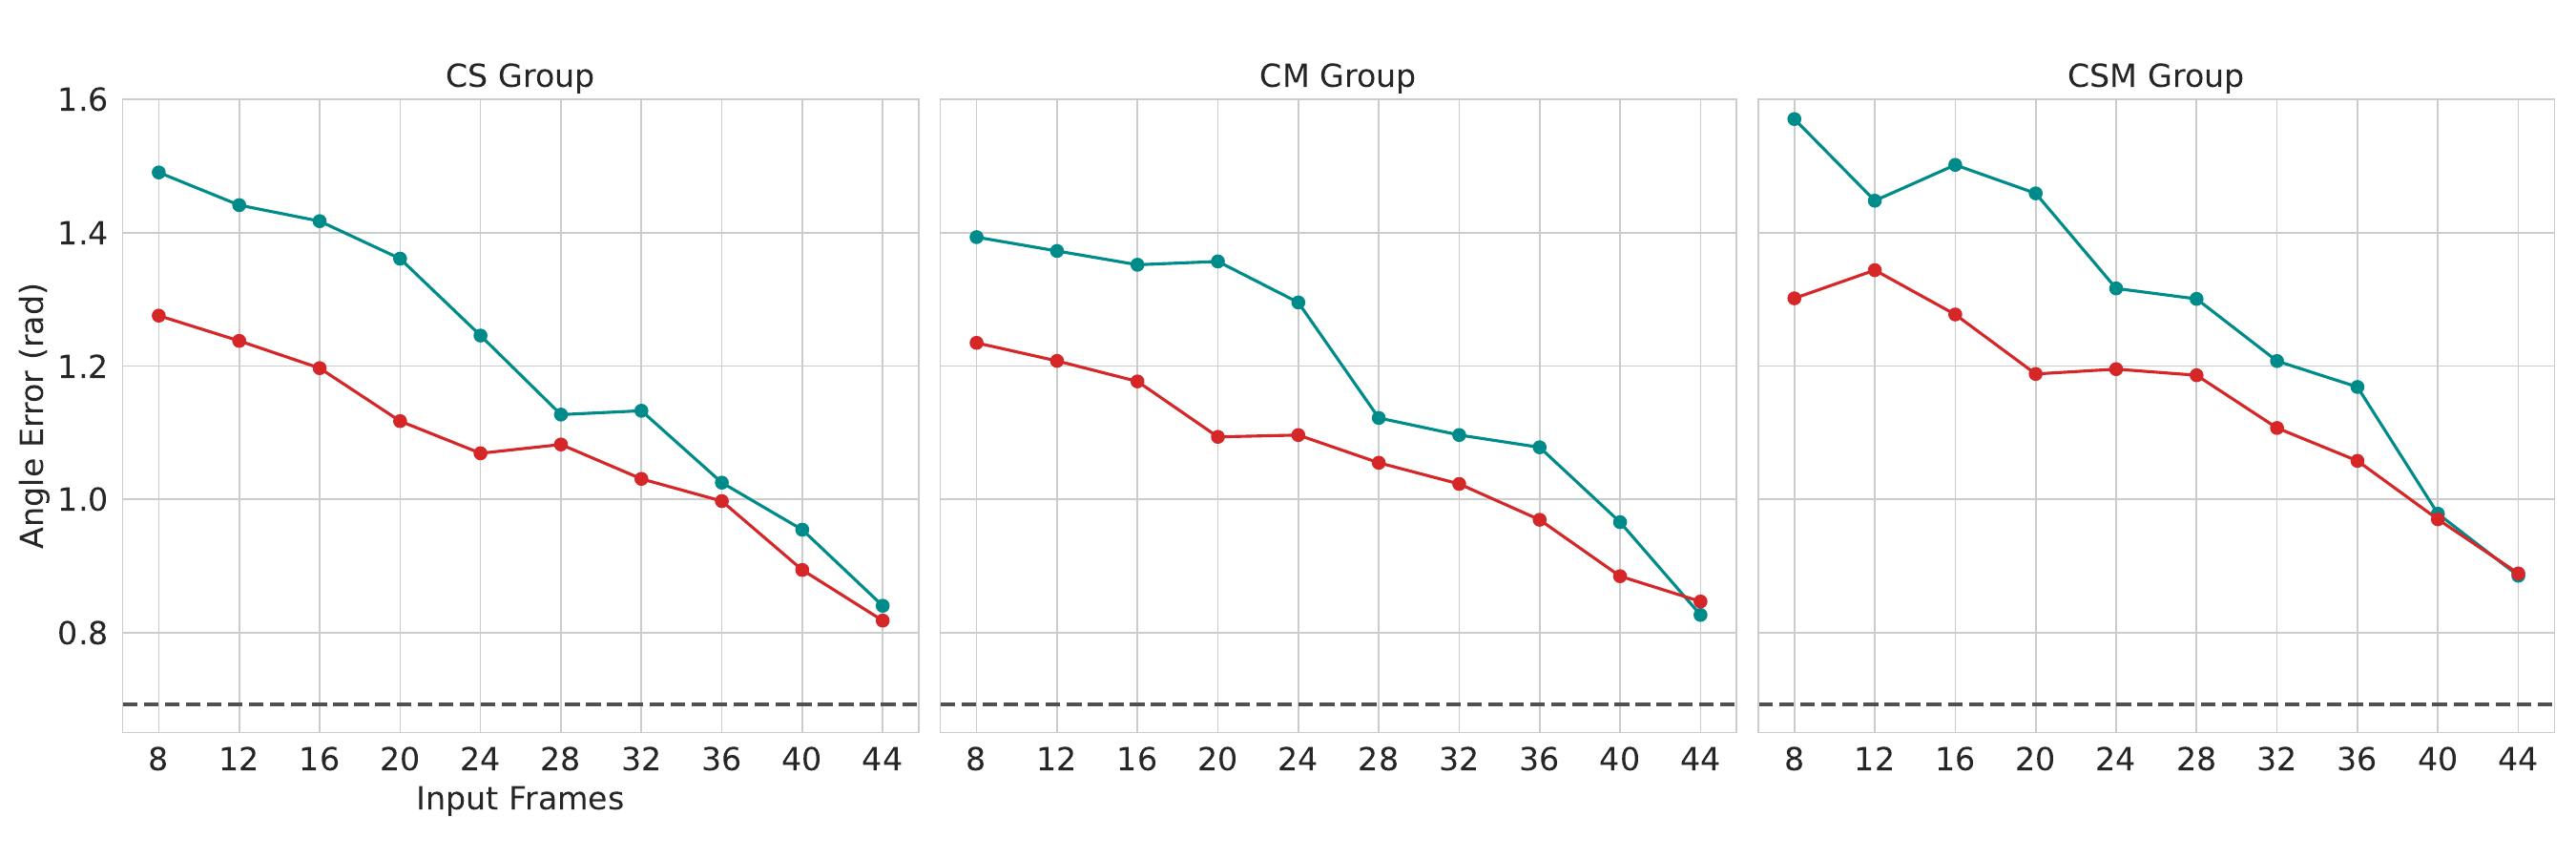}
\caption{\textbf{Key-Pose Angle Error (in $rad$) across Various Input Frames.} This figure displays the MSE for key-pose angle error within the CS, CM, and CSM groups, across different numbers of input frames. Red lines represent results with gaze, and green lines represent results without gaze. Gray dashed lines represent the key-pose angle error calculated directly through the encoder and decoder of the hand-motion VQ-VAE.
}
\label{res_angle}
\end{figure*}

\subsection{Effect of Noise on Hand Joint}
In our previous experiments, data was corrected and smoothed to ensure a noise-free environment. However, noise is inherently present in the dataset collection process. The hand motion data was captured using Aria Glasses RGB camera, which produces a fish-eye output. This, combined with the camera's narrow field of view and instances where the subject moves their head, often results in parts of the hands being occasionally missing or appearing at the very edges of the frame, which can lead to extensive distortion. Additionally, mapping the hand motion into 3D involves significant coordinate transformations, which can influence the reliability and accuracy of hand motion detection. These factors collectively pose challenges to the accuracy of applying such methods in real-time prediction scenarios.

To simulate high noise levels in hand motion estimation, we introduced per-joint Gaussian noise to the system. This noise level and its distribution were chosen based on previous research \cite{salvato2022predhandobj}. We applied Gaussian noise with mean errors of 0.1 m, 0.15 m, 0.2 m, 0.25 m, and 0.3 m, calculating the associated Gaussian standard deviations using the mean of the Chi distribution as follows:
\begin{equation}
\sigma = e \sqrt{\frac{\pi}{8}}
\end{equation}
This noise was independently applied to each joint for every frame. To ensure consistency, the same noise was applied for both models with and without gaze integration at the same timestep. We specifically analyzed the impact of this noise on the shortest input sequence of 8 frames. The results of this analysis are presented in Fig. \ref{res_noise}.

As the noise level rises from 0.1 m to 0.3 m, a consistent increase in both distance and pose errors is observed. The integration of gaze information consistently reduces these distance errors across all groups, demonstrating its effectiveness in noisy conditions. Notably, when the input noise level is below 2.0 m, the distance MSE closely approximates the error observed without noise, illustrating the robustness of the gaze-enhanced model. This indicates the resilience of the gaze-applied model. The benefit of gaze integration becomes more significant with larger noise levels in all groups, contributing significantly to the stability and accuracy of the system in noisy environments. For pose errors, a similar but less pronounced trend is evident. Gaze-enhanced models outperform non-gaze models in the CS group, yet demonstrate a reduced effect in mitigating pose errors within the CM and CSM groups. This suggests that in scenarios involving cross-motion validation, the gaze information is less beneficial for unknown pose accuracy.

\begin{figure*}[htbp]
\centering
\subcaptionbox{Key-Pose Distance Error}{\includegraphics[width=0.95\textwidth]{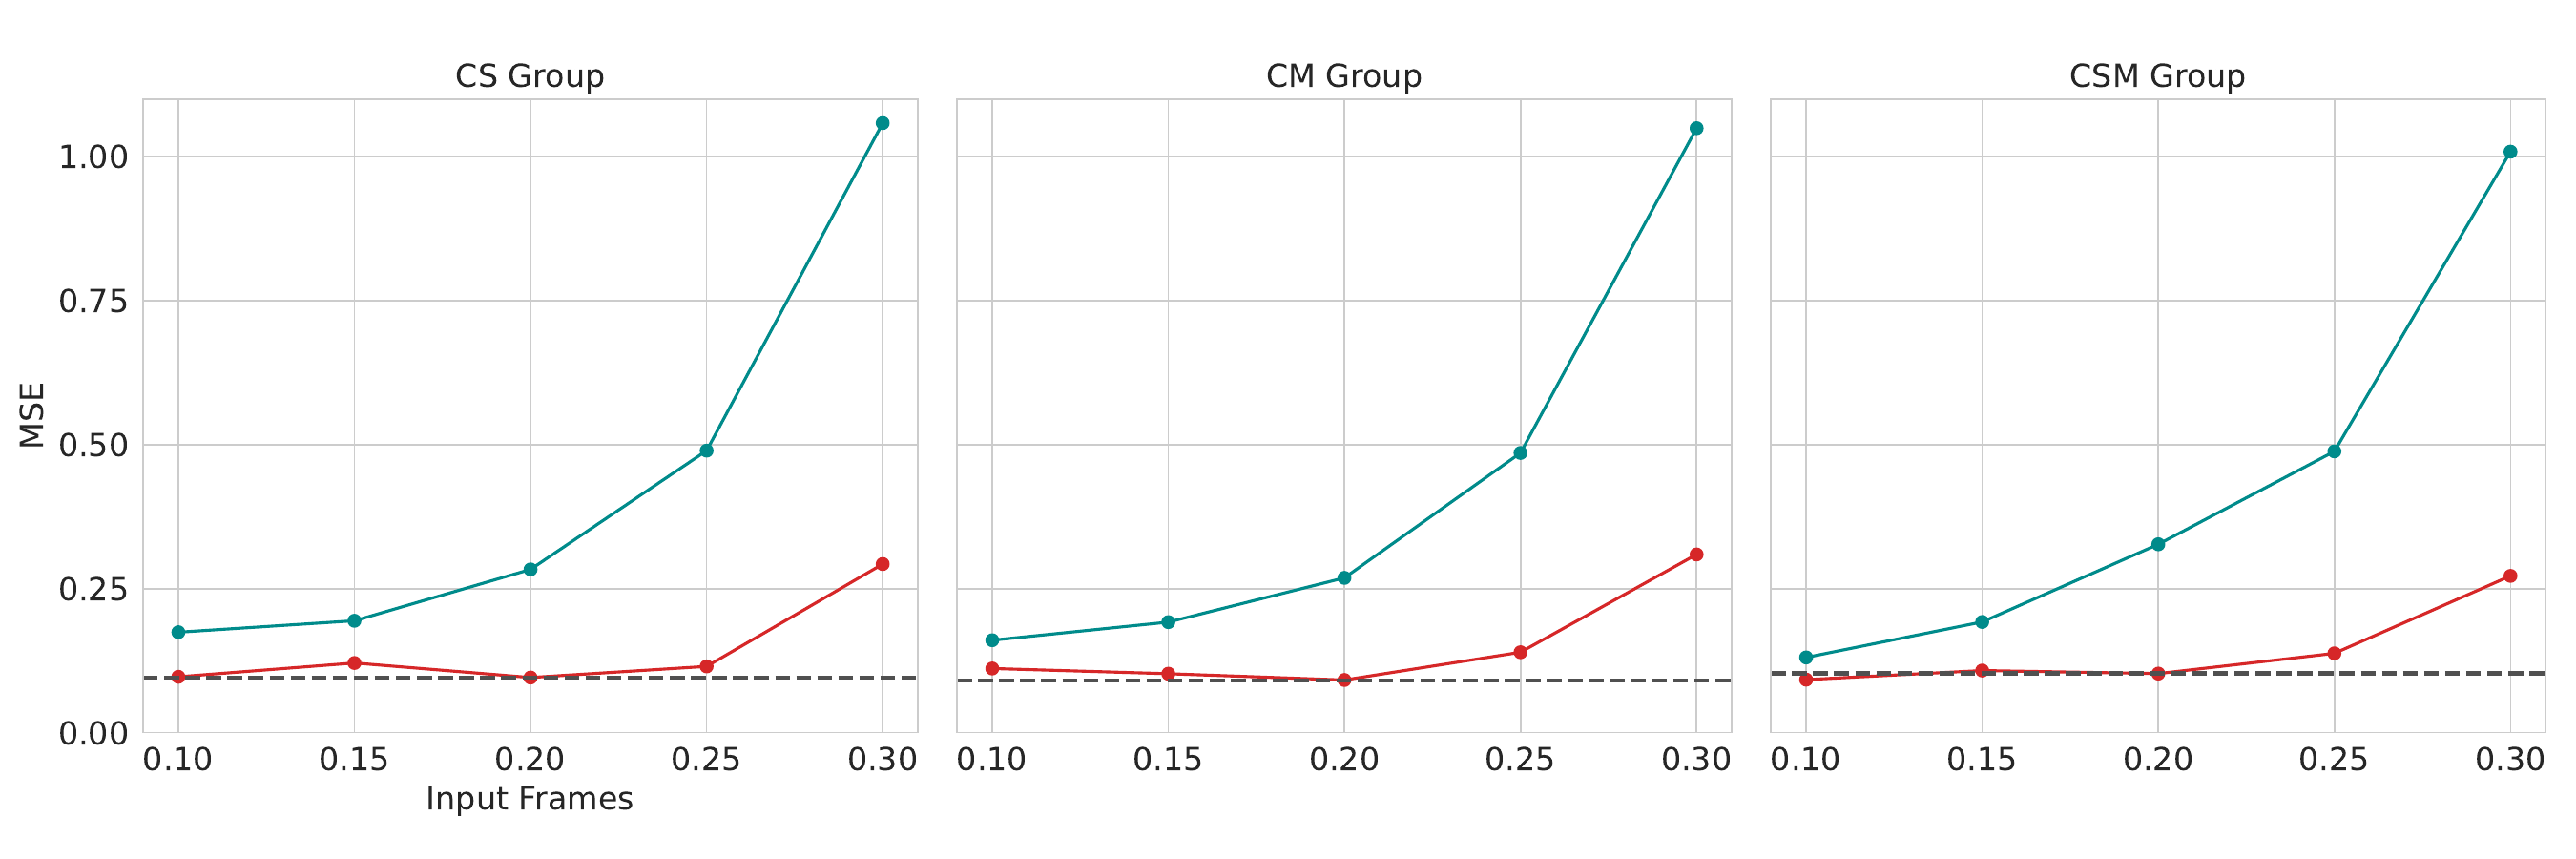}}%
\hfill
\subcaptionbox{Key-Pose Pose Error}{\includegraphics[width=0.95\textwidth]{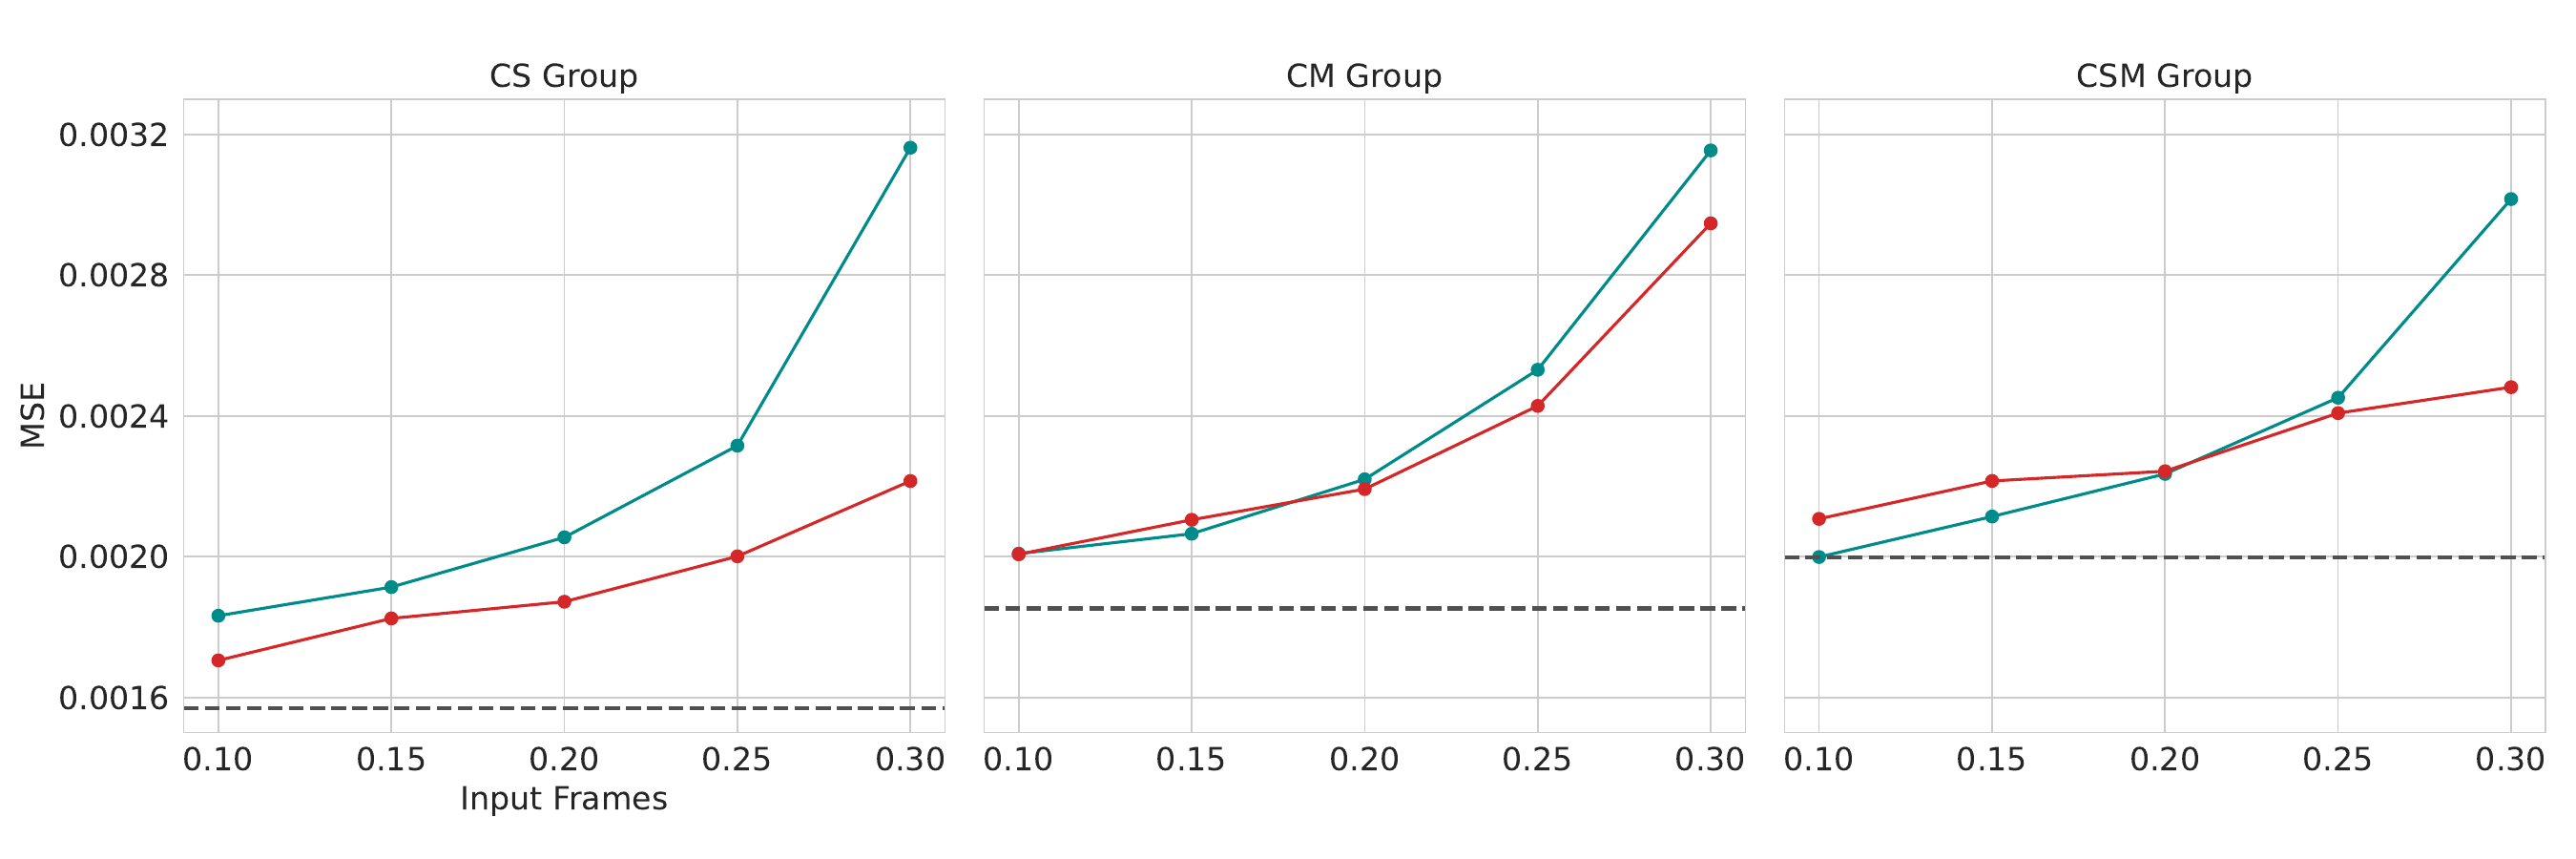}}%
\caption{\textbf{Key-Pose Distance and Pose MSE (in $m^2$) across Different Noise Levels.} This figure displays the MSE for key-pose distance (a) and pose (b) in CS, CM, and CSM groups with 8 input frames. The MSE values for the x, y, and z axes are aggregated. Red lines represent results with gaze, and green lines represent results without gaze. Gray dashed lines indicate, with 8 input frames, the MSE outcomes for key-pose distance and pose when using a gaze-inclusive model without noise, applied for the corresponding group.}
\label{res_noise}
\end{figure*}

\begin{table}[]
\begin{tabular}{l|l|l}
\hline
motion/subject            & 4 folds of subjects & 1 fold of subject        \\ \hline
other                     & train               & cross-subject            \\ 
take book, write on paper & cross-motion        & cross-subject and motion \\ 
\end{tabular}
\end{table}
